# Supplementary material for: Learned Bayesian Cram\'er-Rao Bound for Unknown Measurement Models Using Score Neural Networks
Source: arXiv:2502.00724 source file (2025-02-09)
Supplement: Supplementary file 1 [file unifrom_rolling_off.tex]

\subsection{Uniform Rolling Off}
Here we suggest a uniform rolling off distribution which has the following probability density function, when $\epsilon>0$, $\alpha>1$ and $b>a$

\begin{align}
    \probt{x}{X}=c\begin{cases}
                        \brackets{\frac{b-x}{\epsilon}}^{\alpha}\quad x\in (b-\epsilon,b)\\
                        1\quad x\in [a+\epsilon,b-\epsilon] \\
                        \brackets{\frac{x-a}{\epsilon}}^{\alpha}\quad x \in (a,a+\epsilon)
    \end{cases},
\end{align}
where $c$ is the normalization constant. 
\begin{align}
    u&=\int_{b-\epsilon}^{b}\brackets{\frac{b-x}{\epsilon}}^{\alpha}dx+\int_{a+\epsilon}^{b-\epsilon}dx +\int_{a}^{a+\epsilon}\brackets{\frac{x-a}{\epsilon}}^{\alpha}dx,\nonumber\\
     &=\frac{\epsilon}{\alpha+1}+b-a-2\epsilon+\frac{\epsilon}{\alpha+1}.
\end{align}
then $c=\frac{1}{u}$ and it score function is given by:
\begin{align}
    \nabla_{x}\log\probt{x}{X}=\begin{cases}
                        -\alpha\frac{\epsilon}{b-x}\quad x\in (b-\epsilon,b)\\
                        0\quad x\in [a+\epsilon,b-\epsilon] \\
                        \alpha\frac{\epsilon }{x-a}\quad x \in (a,a+\epsilon)
    \end{cases},
\end{align}
Next, we compute the prior FIM:
\begin{align}
    &\expectation{\brackets{\nabla_{x}\log\probt{x}{X}}^2}{X} =\\
    &c\alpha^{2}\int_{b-\epsilon}^{b}\brackets{\frac{b-x}{\epsilon}}^{\alpha-2}dx+c\int_{a+\epsilon}^{b-\epsilon}1\cdot 0 dx +c\alpha^{2}\int_{a}^{a+\epsilon}\brackets{\frac{x-a}{\epsilon}}^{\alpha-2}dx\\
    &=2c\alpha^{2}\frac{\epsilon}{\alpha-1} .
\end{align}
Finally, to enable sampling we compute the inverse CDF, to do so, we start by computing the CDF which is given by:
\begin{align}
    F_X\brackets{x}= c\begin{cases}
                        \frac{2\epsilon}{\alpha+1}+b-a-2\epsilon-\frac{\epsilon}{\alpha+1}\brackets{\frac{b-x}{\epsilon}}^{\alpha+1}\quad x\in (b-\epsilon,b)\\
                        \frac{\epsilon}{\alpha+1}+x-a-\epsilon\quad x\in [a+\epsilon,b-\epsilon] \\
                        \frac{\epsilon}{\alpha+1}\brackets{\frac{x-a}{\epsilon}}^{\alpha+1}\quad x \in (a,a+\epsilon)
    \end{cases},
\end{align}
and it inverse is given by:

\begin{align}
    F_X^{-1}\brackets{p}=\begin{cases}
                        \frac{2\epsilon}{\alpha+1}+b-a-2\epsilon-\frac{\epsilon}{\alpha+1}\brackets{\frac{b-x}{\epsilon}}^{\alpha+1}\quad x\in (b-\epsilon,b)\\
                        \frac{p}{c}+a+\epsilon-\frac{\epsilon}{\alpha+1}\quad x\in [\frac{c\epsilon}{\alpha+1},1-\frac{c\epsilon}{\alpha+1}] \\
                        a+\epsilon\brackets{\frac{p\brackets{\alpha+1}}{c\epsilon}}^{\frac{1}{\alpha+1}}\quad x \in \brackets{0,\frac{c\epsilon}{\alpha+1}}
    \end{cases},
\end{align}
